# Supplementary material for: Gibbs-Helmholtz Graph Neural Network: capturing the temperature dependency of activity coefficients at infinite dilution
Source: arXiv:2212.01199 ancillary file (2022-12-16)
Supplement: Supplementary file 1 [file SI_v02122022.pdf]

Supplementary Information for

# Gibbs-Helmholtz Graph Neural Network: capturing the temperature dependency of infinite dilution activity coefficients

Edgar Ivan Sanchez Medina, Steffen Linke, Martin Stoll, and Kai Sundmacher\*

\*Corresponding author. E-mail: sundmacher@mpi-magdeburg.mpg.de

## S1 Experimental techniques in the DECHEMA data collection

Percentage of datapoints in the complete DECHEMA data collection obtained by the experimental techniques:

1) Gas-liquid chromatography with gas phase correction (GLCR), 2) Gas-liquid chromatography with no gas phase correction (GLCI), 3) Gas-liquid chromatography with no specification of gas phase correction (GLCN), 4) Derived from solubility data (SOLU), 5) Dilutor technique (DILU), 6) Static method (STAT), 7) Ebulliometry (EBUL) and 8) other techniques (e.g., liquid-liquid chromatography, derived from Henry coefficients, non-steady-state gas-liquid chromatography, isopiestic technique, dew point technique, relative gas-liquid chromatography and Rayleigh distillation method) (OTHR).

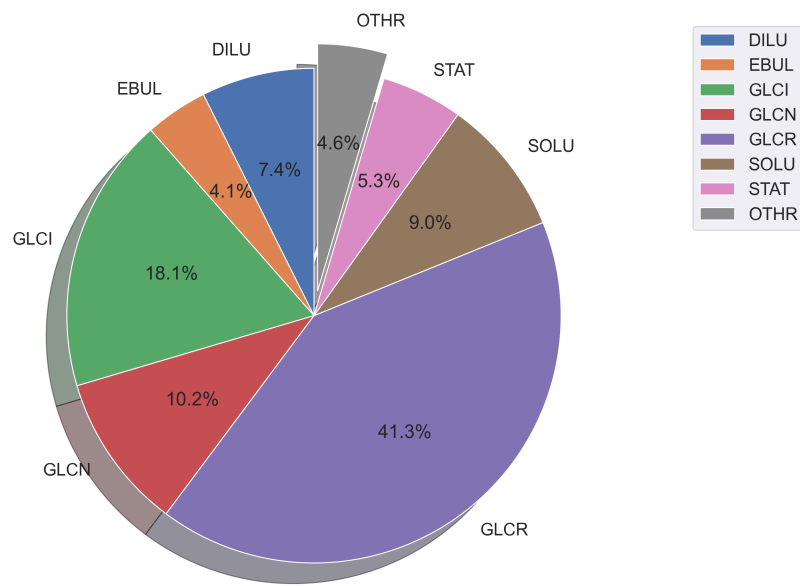

**Figure S1:** Percentage of datapoints on the complete DECHEMA data collection obtained by different experimental techniques.

## S2 Temperature distribution on the DECHEMA dataset

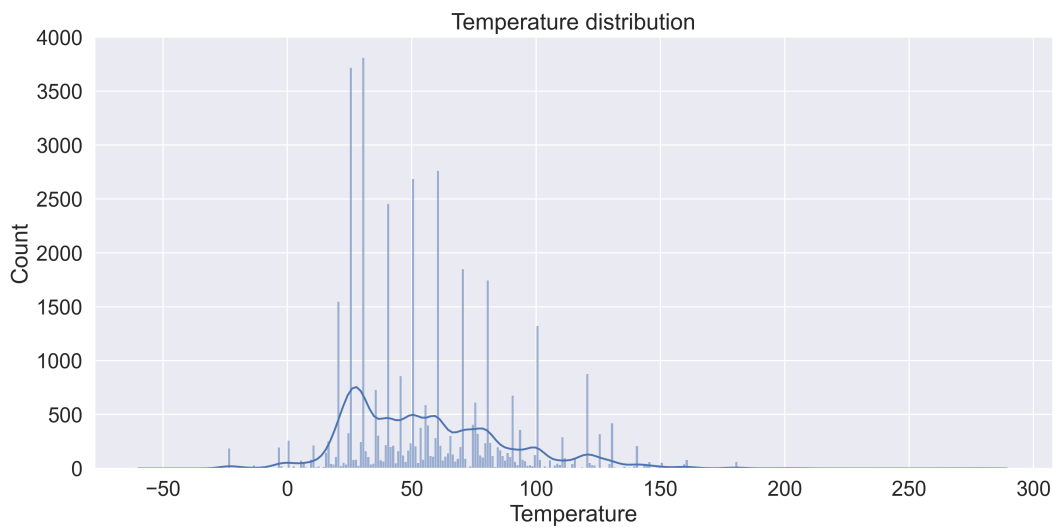

**Figure S2:** Distribution of temperature values covered in the DECHEMA dataset.

## S3 Infinite dilution activity coefficient distribution on the DECHEMA dataset

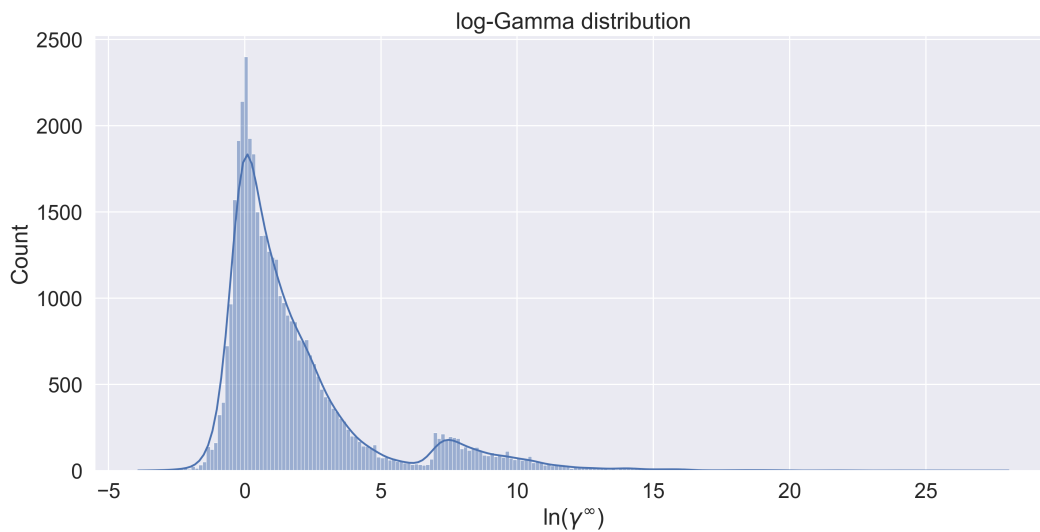

**Figure S3:** Distribution of  $\ln \gamma_{ij}^{\infty}$  values covered in the DECHEMA dataset.

## S4 Chemical classes contained in the DECHEMA dataset

These chemical classes were obtained by the Classyfire tool [1] which, to the best of our knowledge, provides the largest and most consistent taxonomy across the chemical space.

**Table S1:** Chemical classes contained in the DECHEMA dataset obtained from the Classyfire tool [1] along the number of chemical species contained in each class.

| Class                                    | No. | Class                                    | No. |
|------------------------------------------|-----|------------------------------------------|-----|
| Benzene and substituted derivatives      | 271 | Phenanthrenes and derivatives            | 4   |
| Organooxygen compounds                   | 193 | Lactams                                  | 4   |
| Fatty Acyls                              | 136 | Epoxides                                 | 4   |
| Organonitrogen compounds                 | 113 | Keto acids and derivatives               | 3   |
| Carboxylic acids and derivatives         | 104 | Sulfonyls                                | 3   |
| Saturated hydrocarbons                   | 103 | Other non-metal organides                | 3   |
| Unsaturated hydrocarbons                 | 67  | Azobenzenes                              | 3   |
| Prenol lipids                            | 39  | Dioxanes                                 | 3   |
| Organofluorides                          | 32  | Homogeneous other non-metal compounds    | 3   |
| Phenols                                  | 30  | Pyrroles                                 | 3   |
| Organochlorides                          | 28  | Oxanes                                   | 2   |
| Alkyl halides                            | 27  | Dioxolanes                               | 2   |
| Pyridines and derivatives                | 22  | Dihydrofurans                            | 2   |
| Phenol ethers                            | 22  | Depsidic acids and depsidones            | 2   |
| Naphthalenes                             | 20  | Thiophenes                               | 2   |
| Organobromides                           | 19  | Hydroxy acids and derivatives            | 2   |
| Allyl-type 1,3-dipolar organic compounds | 19  | Organic sulfonic acids and derivatives   | 2   |
| Organic phosphoric acids and derivatives | 12  | Oxolanes                                 | 2   |
| Quinolines and derivatives               | 12  | Organic phosphonic acids and derivatives | 2   |
| Thioethers                               | 12  | Fluorenes                                | 2   |
| Vinyl halides                            | 12  | Organic sulfuric acids and derivatives   | 2   |
| Thiols                                   | 11  | Oxathiolanes                             | 2   |
| Heteroaromatic compounds                 | 11  | Indoles and derivatives                  | 2   |
| Pyrrolidines                             | 11  | Oxathianes                               | 2   |
| Organoiodides                            | 10  | Stilbenes                                | 1   |
| Halohydrins                              | 10  | Acyl halides                             | 1   |
| Organic oxoanionic compounds             | 9   | Thiophenols                              | 1   |
| Lactones                                 | 9   | Diarylheptanoids                         | 1   |

|                                        |   |                                        |   |
|----------------------------------------|---|----------------------------------------|---|
| Piperidines                            | 9 | Isoquinolines and derivatives          | 1 |
| Furans                                 | 9 | Benzofurans                            | 1 |
| Azolidines                             | 9 | Aziridines                             | 1 |
| Organo-post-transition metal compounds | 9 | Organophosphinic acids and derivatives | 1 |
| Organometalloid compounds              | 8 | Homogeneous halogens                   | 1 |
| Phenol esters                          | 8 | Homogeneous transition metal compounds | 1 |
| Oxazinanes                             | 8 | Pyrenes                                | 1 |
| Tetrahydrofurans                       | 7 | Anthracenes                            | 1 |
| Thiolanes                              | 6 | Indanes                                | 1 |
| Azoles                                 | 6 | Benzothiophenes                        | 1 |
| Sulfoxides                             | 6 | Oxacyclic compounds                    | 1 |
| Polycyclic hydrocarbons                | 6 | Tetalins                               | 1 |
| Glycerolipids                          | 6 | Indenes and isoindenes                 | 1 |
| Organic carbonic acids and derivatives | 5 | Organic disulfides                     | 1 |
| Carboximidic acids and derivatives     | 5 | Trialkylphosphites                     | 1 |
| Organic oxides                         | 5 | Acyclic allenes                        | 1 |
| Aryl halides                           | 5 | Organic metal salts                    | 1 |
| Diazinanes                             | 4 |                                        |   |

## S5 Hyperparameters for GNNprevious in the isothermal studies

The hyperparameters for GNNprevious were tuned using Optuna [2] by setting the number of trials to 100 and using the corresponding ranges and scales shown in Table S2. For hyperparameter tuning 10-fold cross-validation was used. The final hyperparameters selected for each isothermal study are shown in Table S3. The loss function used was Mean Squared Error (MSE).

**Table S2:** Ranges used during the hyperparameter search of GNNprevious in the isothermal studies.

| Hyperparameter           | Range                     | Search scale |
|--------------------------|---------------------------|--------------|
| Message passing layers   | 2-5                       | integer      |
| Dropout ratio            | 0.05-0.5                  | uniform      |
| Hidden embedding size    | 16-256                    | integer      |
| Learning rate            | 0.0001-1                  | loguniform   |
| Units in message passing | 8-64                      | integer      |
| Epochs                   | 100-300                   | integer      |
| Batch size               | 4-64                      | integer      |
| Jumping knowledge        | {last, sum, mean}         | categorical  |
| Global pooling           | {sum, mean, max, set2set} | categorical  |
| Hidden layers final MLP  | 1-2                       | integer      |
| Units in final MLP       | 16-128                    | integer      |

**Table S3:** Final selected hyperparameters for GNNprevious in each isothermal study.

| Hyperparameter           | Final value for T (°) |        |         |          |          |          |         |        |         |
|--------------------------|-----------------------|--------|---------|----------|----------|----------|---------|--------|---------|
|                          | 20                    | 25     | 30      | 40       | 50       | 60       | 70      | 80     | 100     |
| Message passing layers   | 4                     | 3      | 4       | 2        | 3        | 3        | 4       | 3      | 5       |
| Dropout ratio            | 0.13                  | 0.05   | 0.13    | 0.05     | 0.05     | 0.06     | 0.05    | 0.07   | 0.07    |
| Hidden embedding size    | 234                   | 41     | 154     | 209      | 72       | 88       | 250     | 64     | 30      |
| Learning rate            | 0.002                 | 0.002  | 0.011   | 0.003    | 0.002    | 0.011    | 0.001   | 0.007  | 0.009   |
| Units in message passing | 21                    | 31     | 18      | 37       | 12       | 42       | 37      | 39     | 10      |
| Epochs                   | 188                   | 239    | 274     | 238      | 168      | 289      | 226     | 144    | 256     |
| Batch size               | 39                    | 59     | 62      | 44       | 53       | 44       | 42      | 53     | 62      |
| Jumping knowledge        | last                  | sum    | mean    | mean     | mean     | mean     | sum     | mean   | mean    |
| Global pooling           | sum                   | sum    | set2set | sum      | sum      | sum      | sum     | sum    | mean    |
| Hidden layers final MLP  | 2                     | 2      | 1       | 2        | 2        | 2        | 2       | 2      | 2       |
| Units in final MLP       | 105, 74               | 83, 30 | 125     | 110, 112 | 104, 126 | 113, 122 | 105, 18 | 97, 56 | 100, 30 |

## S6 Hyperparameters for SolvGNN in the isothermal studies

The hyperparameters for SolvGNN were tuned using Optuna [2] by setting the number of trials to 100 and using the corresponding ranges and scales shown in Table S4. For hyperparameter tuning 10-fold cross-validation was used. The final hyperparameters selected for each isothermal study are shown in Table S5. The loss function used was Mean Squared Error (MSE).

**Table S4:** Ranges used during the hyperparameter search of SolvGNN in the isothermal studies.

| Hyperparameter        | Range    | Search scale |
|-----------------------|----------|--------------|
| Hidden embedding size | 16-256   | integer      |
| Learning rate         | 0.0001-1 | loguniform   |
| Epochs                | 100-300  | integer      |
| Batch size            | 4-64     | integer      |

**Table S5:** Final selected hyperparameters for SolvGNN in each isothermal study.

| Hyperparameter        | Final value for T (°) |        |        |        |        |        |        |        |        |
|-----------------------|-----------------------|--------|--------|--------|--------|--------|--------|--------|--------|
|                       | 20                    | 25     | 30     | 40     | 50     | 60     | 70     | 80     | 100    |
| Hidden embedding size | 242                   | 226    | 236    | 186    | 197    | 182    | 252    | 162    | 177    |
| Learning rate         | 0.0004                | 0.0004 | 0.0001 | 0.0002 | 0.0006 | 0.0003 | 0.0006 | 0.0002 | 0.0006 |
| Epochs                | 156                   | 178    | 287    | 151    | 212    | 299    | 256    | 254    | 260    |
| Batch size            | 5                     | 12     | 4      | 4      | 9      | 7      | 8      | 4      | 4      |

## S7 Hyperparameters for GH-GNN and SolvGNNGH in the temperature dependency studies

The hyperparameters for GH-GNN and SolvGNNGH were tuned using Optuna [2] by setting the number of trials to 100, the number of epochs to 50 and using the corresponding ranges and scales shown in Tables S6 and S7. The final hyperparameters selected are also shown in Tables S6 and S7, correspondingly. For hyperparameter tuning 10-fold cross-validation was used. After the other hyperparameters were selected, the number of epochs were varied over the shown values to select the one that improves the performance on the validation set. The loss function used was Mean Squared Error (MSE).

**Table S6:** Ranges used during the hyperparameter search of GH-GNN in the temperature dependency studies. The number of epochs was set to 50 for each trial.

| Hyperparameter        | Range                     | Search scale | Selected value |
|-----------------------|---------------------------|--------------|----------------|
| Hidden embedding size | 16-128                    | integer      | 113            |
| Learning rate         | 0.0001-1                  | loguniform   | 0.0002         |
| Epochs                | {100, 150, 200, 250, 300} | categorical  | 250            |
| Batch size            | 4-64                      | integer      | 32             |

**Table S7:** Ranges used during the hyperparameter search of SolvGNNGH in the temperature dependency studies. The number of epochs was set to 50 for each trial.

| Hyperparameter        | Range                     | Search scale | Selected value |
|-----------------------|---------------------------|--------------|----------------|
| Hidden embedding size | 16-128                    | integer      | 128            |
| Learning rate         | 0.0001-1                  | loguniform   | 0.0005         |
| Epochs                | {100, 150, 200, 250, 300} | categorical  | 300            |
| Batch size            | 4-64                      | integer      | 23             |

## S8 Binary systems used for training GH-GNN

Collection of all solvent-solute chemical classes contained in the training set used for developing the GH-GNN model. According to the discussion of the results section in the paper regarding the discrete extrapolation, systems with more than 25 occurrences are expected to produce results with a MAE of approximately 0.3. This systems are marked with a star. “NA” denotes that the class for such compound is “Not-available” according to Classyfire [1].

**Table S8:** Binary solvent-solute classes contained in the training set used for developing GH-GNN and their occurrences.

| No. | Solvent-solute chemical classes                                             | Systems |
|-----|-----------------------------------------------------------------------------|---------|
| 1   | * Benzene and substituted derivatives–Saturated hydrocarbons                | 876     |
| 2   | * Organooxygen compounds–Saturated hydrocarbons                             | 596     |
| 3   | * Benzene and substituted derivatives–Benzene and substituted derivatives   | 450     |
| 4   | * Saturated hydrocarbons–Saturated hydrocarbons                             | 395     |
| 5   | * Organooxygen compounds–Organooxygen compounds                             | 307     |
| 6   | * Organonitrogen compounds–Saturated hydrocarbons                           | 297     |
| 7   | * Fatty Acyls–Saturated hydrocarbons                                        | 258     |
| 8   | * Organooxygen compounds–Benzene and substituted derivatives                | 245     |
| 9   | * Saturated hydrocarbons–Organooxygen compounds                             | 237     |
| 10  | * Organooxygen compounds–Unsaturated hydrocarbons                           | 227     |
| 11  | * Benzene and substituted derivatives–Organooxygen compounds                | 221     |
| 12  | * Benzene and substituted derivatives–Unsaturated hydrocarbons              | 218     |
| 13  | * Carboxylic acids and derivatives–Saturated hydrocarbons                   | 212     |
| 14  | * Fatty Acyls–Organooxygen compounds                                        | 161     |
| 15  | * Homogeneous other non-metal compounds–Organooxygen compounds              | 147     |
| 16  | * Organonitrogen compounds–Unsaturated hydrocarbons                         | 143     |
| 17  | * Saturated hydrocarbons–Benzene and substituted derivatives                | 134     |
| 18  | * Homogeneous other non-metal compounds–Benzene and substituted derivatives | 111     |
| 19  | * Organonitrogen compounds–Benzene and substituted derivatives              | 109     |
| 20  | * Allyl-type 1,3-dipolar organic compounds–Saturated hydrocarbons           | 108     |
| 21  | * Fatty Acyls–Benzene and substituted derivatives                           | 108     |
| 22  | * Carboxylic acids and derivatives–Benzene and substituted derivatives      | 102     |
| 23  | * Saturated hydrocarbons–Unsaturated hydrocarbons                           | 95      |
| 24  | * Naphthalenes–Saturated hydrocarbons                                       | 93      |
| 25  | * Organooxygen compounds–Alkyl halides                                      | 93      |

|    |                                                                          |    |
|----|--------------------------------------------------------------------------|----|
| 26 | * Benzene and substituted derivatives–Alkyl halides                      | 90 |
| 27 | * Quinolines and derivatives–Saturated hydrocarbons                      | 89 |
| 28 | * Carboxylic acids and derivatives–Unsaturated hydrocarbons              | 86 |
| 29 | * Fatty Acyls–Carboxylic acids and derivatives                           | 83 |
| 30 | * Organooxygen compounds–Carboxylic acids and derivatives                | 81 |
| 31 | * Organo-post-transition metal compounds–Saturated hydrocarbons          | 81 |
| 32 | * Carboxylic acids and derivatives–Organooxygen compounds                | 78 |
| 33 | * Homogeneous other non-metal compounds–Fatty Acyls                      | 77 |
| 34 | * Organooxygen compounds–Organochlorides                                 | 76 |
| 35 | * Pyrrolidines–Saturated hydrocarbons                                    | 75 |
| 36 | * Fatty Acyls–Unsaturated hydrocarbons                                   | 74 |
| 37 | * Pyrrolidines–Unsaturated hydrocarbons                                  | 70 |
| 38 | * Organonitrogen compounds–Organooxygen compounds                        | 70 |
| 39 | * Homogeneous other non-metal compounds–Carboxylic acids and derivatives | 68 |
| 40 | * Pyridines and derivatives–Saturated hydrocarbons                       | 68 |
| 41 | * Phenol ethers–Saturated hydrocarbons                                   | 68 |
| 42 | * Saturated hydrocarbons–Carboxylic acids and derivatives                | 66 |
| 43 | * Oxazinanes–Saturated hydrocarbons                                      | 64 |
| 44 | * Saturated hydrocarbons–Organochlorides                                 | 62 |
| 45 | * Benzene and substituted derivatives–Organochlorides                    | 62 |
| 46 | * Carboximidic acids and derivatives–Organooxygen compounds              | 61 |
| 47 | * Thiolanes–Saturated hydrocarbons                                       | 59 |
| 48 | * Organic phosphoric acids and derivatives–Saturated hydrocarbons        | 58 |
| 49 | * Homogeneous other non-metal compounds–Saturated hydrocarbons           | 57 |
| 50 | * Benzene and substituted derivatives–Carboxylic acids and derivatives   | 56 |
| 51 | * Phenols–Saturated hydrocarbons                                         | 55 |
| 52 | * Oxazinanes–Unsaturated hydrocarbons                                    | 55 |
| 53 | * Fatty Acyls–Alkyl halides                                              | 54 |
| 54 | * Fatty Acyls–Organochlorides                                            | 54 |
| 55 | * Pyrrolidines–Organooxygen compounds                                    | 53 |
| 56 | * Organic phosphoric acids and derivatives–Organooxygen compounds        | 53 |
| 57 | * Saturated hydrocarbons–Organonitrogen compounds                        | 52 |
| 58 | * Halohydrins–Saturated hydrocarbons                                     | 50 |
| 59 | * Furans–Saturated hydrocarbons                                          | 49 |
| 60 | * Homogeneous other non-metal compounds–Organonitrogen compounds         | 49 |
| 61 | * Quinolines and derivatives–Benzene and substituted derivatives         | 48 |

|    |                                                                                |    |
|----|--------------------------------------------------------------------------------|----|
| 62 | * Sulfoxides–Saturated hydrocarbons                                            | 46 |
| 63 | * Saturated hydrocarbons–Alkyl halides                                         | 45 |
| 64 | * Prenol lipids–Saturated hydrocarbons                                         | 44 |
| 65 | * Unsaturated hydrocarbons–Benzene and substituted derivatives                 | 44 |
| 66 | * Prenol lipids–Organooxygen compounds                                         | 43 |
| 67 | * Piperidines–Saturated hydrocarbons                                           | 42 |
| 68 | * Saturated hydrocarbons–Homogeneous other non-metal compounds                 | 42 |
| 69 | * Organooxygen compounds–Organonitrogen compounds                              | 40 |
| 70 | * Benzene and substituted derivatives–Organonitrogen compounds                 | 39 |
| 71 | * Alkyl halides–Saturated hydrocarbons                                         | 39 |
| 72 | * Carboximidic acids and derivatives–Saturated hydrocarbons                    | 39 |
| 73 | * Azolidines–Unsaturated hydrocarbons                                          | 38 |
| 74 | * Unsaturated hydrocarbons–Saturated hydrocarbons                              | 37 |
| 75 | * Lactams–Saturated hydrocarbons                                               | 35 |
| 76 | * Azolidines–Saturated hydrocarbons                                            | 35 |
| 77 | * Piperidines–Unsaturated hydrocarbons                                         | 32 |
| 78 | * Tetrahydrofurans–Saturated hydrocarbons                                      | 32 |
| 79 | * Sulfoxides–Unsaturated hydrocarbons                                          | 31 |
| 80 | * Unsaturated hydrocarbons–Organooxygen compounds                              | 31 |
| 81 | * Allyl-type 1,3-dipolar organic compounds–Benzene and substituted derivatives | 31 |
| 82 | * Organic phosphoric acids and derivatives–Benzene and substituted derivatives | 31 |
| 83 | * Organonitrogen compounds–Alkyl halides                                       | 31 |
| 84 | * Azoles–Saturated hydrocarbons                                                | 31 |
| 85 | * Fatty Acyls–Organonitrogen compounds                                         | 31 |
| 86 | * Organonitrogen compounds–Organochlorides                                     | 30 |
| 87 | * Phenanthrenes and derivatives–Benzene and substituted derivatives            | 29 |
| 88 | * Naphthalenes–Benzene and substituted derivatives                             | 29 |
| 89 | * Carboximidic acids and derivatives–Unsaturated hydrocarbons                  | 29 |
| 90 | * Organochlorides–Saturated hydrocarbons                                       | 28 |
| 91 | * Organooxygen compounds–Homogeneous other non-metal compounds                 | 28 |
| 92 | * Organofluorides–Saturated hydrocarbons                                       | 28 |
| 93 | * Phenol ethers–Benzene and substituted derivatives                            | 27 |
| 94 | * Organochlorides–Organooxygen compounds                                       | 27 |
| 95 | * Thioethers–Saturated hydrocarbons                                            | 26 |
| 96 | * Pyridines and derivatives–Benzene and substituted derivatives                | 26 |
| 97 | * Saturated hydrocarbons–Pyridines and derivatives                             | 26 |

|     |                                                                              |    |
|-----|------------------------------------------------------------------------------|----|
| 98  | * Organooxygen compounds–Organofluorides                                     | 26 |
| 99  | * Organochlorides–Benzene and substituted derivatives                        | 26 |
| 100 | * Homogeneous other non-metal compounds–Phenols                              | 26 |
| 101 | * Prenol lipids–Benzene and substituted derivatives                          | 26 |
| 102 | * Diarylheptanoids–Benzene and substituted derivatives                       | 25 |
| 103 | * Thiolanes–Benzene and substituted derivatives                              | 25 |
| 104 | * Thiolanes–Unsaturated hydrocarbons                                         | 25 |
| 105 | * Furans–Unsaturated hydrocarbons                                            | 25 |
| 106 | Saturated hydrocarbons–Organobromides                                        | 24 |
| 107 | Heteroaromatic compounds–Saturated hydrocarbons                              | 24 |
| 108 | Carboxylic acids and derivatives–Alkyl halides                               | 24 |
| 109 | Thiolanes–Organooxygen compounds                                             | 23 |
| 110 | Homogeneous other non-metal compounds–Unsaturated hydrocarbons               | 23 |
| 111 | Glycerolipids–Organooxygen compounds                                         | 23 |
| 112 | Alkyl halides–Organooxygen compounds                                         | 23 |
| 113 | Pyrrolidines–Benzene and substituted derivatives                             | 22 |
| 114 | Organic carbonic acids and derivatives–Organooxygen compounds                | 22 |
| 115 | Saturated hydrocarbons–Fatty Acyls                                           | 22 |
| 116 | Saturated hydrocarbons–Allyl-type 1,3-dipolar organic compounds              | 22 |
| 117 | Organic phosphoric acids and derivatives–Carboxylic acids and derivatives    | 21 |
| 118 | Allyl-type 1,3-dipolar organic compounds–Unsaturated hydrocarbons            | 21 |
| 119 | Organooxygen compounds–Dioxanes                                              | 21 |
| 120 | Homogeneous other non-metal compounds–Organochlorides                        | 21 |
| 121 | Organofluorides–Organooxygen compounds                                       | 21 |
| 122 | Organonitrogen compounds–Thioethers                                          | 20 |
| 123 | Benzene and substituted derivatives–Allyl-type 1,3-dipolar organic compounds | 20 |
| 124 | Prenol lipids–Unsaturated hydrocarbons                                       | 20 |
| 125 | Carboxylic acids and derivatives–Carboxylic acids and derivatives            | 20 |
| 126 | Diazinanes–Saturated hydrocarbons                                            | 20 |
| 127 | Organooxygen compounds–Allyl-type 1,3-dipolar organic compounds              | 20 |
| 128 | Lactones–Saturated hydrocarbons                                              | 20 |
| 129 | Glycerolipids–Prenol lipids                                                  | 19 |
| 130 | Organonitrogen compounds–Carboxylic acids and derivatives                    | 19 |
| 131 | Carboximide acids and derivatives–Benzene and substituted derivatives        | 18 |
| 132 | Organic phosphoric acids and derivatives–Unsaturated hydrocarbons            | 18 |
| 133 | Lactams–Unsaturated hydrocarbons                                             | 18 |

|     |                                                                            |    |
|-----|----------------------------------------------------------------------------|----|
| 134 | NA–Saturated hydrocarbons                                                  | 18 |
| 135 | Organic carbonic acids and derivatives–Benzene and substituted derivatives | 17 |
| 136 | Organonitrogen compounds–Organonitrogen compounds                          | 17 |
| 137 | Depsidones–Saturated hydrocarbons                                          | 17 |
| 138 | Organic metal salts–Saturated hydrocarbons                                 | 17 |
| 139 | Phenols–Benzene and substituted derivatives                                | 17 |
| 140 | Diazinanes–Unsaturated hydrocarbons                                        | 17 |
| 141 | Organobromides–Saturated hydrocarbons                                      | 17 |
| 142 | Oxazinanes–Benzene and substituted derivatives                             | 17 |
| 143 | Organo-post-transition metal compounds–Benzene and substituted derivatives | 17 |
| 144 | Oxazinanes–Organooxygen compounds                                          | 16 |
| 145 | Dioxanes–Saturated hydrocarbons                                            | 16 |
| 146 | Organooxygen compounds–Naphthalenes                                        | 16 |
| 147 | Isoquinolines and derivatives–Saturated hydrocarbons                       | 16 |
| 148 | Organochlorides–Organochlorides                                            | 16 |
| 149 | Unsaturated hydrocarbons–Unsaturated hydrocarbons                          | 16 |
| 150 | Organochlorides–Alkyl halides                                              | 16 |
| 151 | Carboximide acids and derivatives–Carboxylic acids and derivatives         | 16 |
| 152 | Lactones–Organooxygen compounds                                            | 16 |
| 153 | Saturated hydrocarbons–NA                                                  | 15 |
| 154 | Benzene and substituted derivatives–Fatty Acyls                            | 15 |
| 155 | Azoles–Unsaturated hydrocarbons                                            | 15 |
| 156 | Saturated hydrocarbons–Organofluorides                                     | 15 |
| 157 | Organic phosphoric acids and derivatives–Alkyl halides                     | 15 |
| 158 | Unsaturated hydrocarbons–Carboxylic acids and derivatives                  | 15 |
| 159 | Phenol ethers–Unsaturated hydrocarbons                                     | 14 |
| 160 | Piperidines–Organooxygen compounds                                         | 14 |
| 161 | Organic carbonic acids and derivatives–Saturated hydrocarbons              | 14 |
| 162 | Benzene and substituted derivatives–Heteroaromatic compounds               | 14 |
| 163 | Lactams–Benzene and substituted derivatives                                | 14 |
| 164 | Naphthalenes–Unsaturated hydrocarbons                                      | 14 |
| 165 | Diarylheptanoids–Saturated hydrocarbons                                    | 14 |
| 166 | Alkyl halides–Benzene and substituted derivatives                          | 14 |
| 167 | Organooxygen compounds–Fatty Acyls                                         | 14 |
| 168 | Homogeneous other non-metal compounds–Alkyl halides                        | 14 |
| 169 | Azolidines–Organooxygen compounds                                          | 14 |

|     |                                                               |    |
|-----|---------------------------------------------------------------|----|
| 170 | Homogeneous other non-metal compounds–Prenol lipids           | 13 |
| 171 | NA–Unsaturated hydrocarbons                                   | 13 |
| 172 | Prenol lipids–Organochlorides                                 | 13 |
| 173 | Prenol lipids–Carboxylic acids and derivatives                | 13 |
| 174 | Tetrahydrofurans–Unsaturated hydrocarbons                     | 13 |
| 175 | Naphthalenes–Organooxygen compounds                           | 13 |
| 176 | Saturated hydrocarbons–Organoiodides                          | 13 |
| 177 | Sulfoxides–Organooxygen compounds                             | 13 |
| 178 | Prenol lipids–Pyridines and derivatives                       | 13 |
| 179 | NA–Organooxygen compounds                                     | 13 |
| 180 | Organobromides–Benzene and substituted derivatives            | 13 |
| 181 | Sulfonyls–Saturated hydrocarbons                              | 13 |
| 182 | Prenol lipids–Alkyl halides                                   | 13 |
| 183 | Benzene and substituted derivatives–Dioxanes                  | 12 |
| 184 | Organometalloid compounds–Saturated hydrocarbons              | 12 |
| 185 | Sulfoxides–Benzene and substituted derivatives                | 12 |
| 186 | Organooxygen compounds–Organo-post-transition metal compounds | 12 |
| 187 | Halohydrins–Unsaturated hydrocarbons                          | 12 |
| 188 | Prenol lipids–Heteroaromatic compounds                        | 12 |
| 189 | Quinolines and derivatives–Unsaturated hydrocarbons           | 12 |
| 190 | Benzene and substituted derivatives–Vinyl halides             | 12 |
| 191 | Depsides and depsidones–Benzene and substituted derivatives   | 12 |
| 192 | Alkyl halides–Organochlorides                                 | 12 |
| 193 | Organooxygen compounds–Vinyl halides                          | 12 |
| 194 | Sulfonyls–Unsaturated hydrocarbons                            | 11 |
| 195 | Azobenzenes–Benzene and substituted derivatives               | 11 |
| 196 | Organooxygen compounds–Heteroaromatic compounds               | 11 |
| 197 | Organonitrogen compounds–NA                                   | 11 |
| 198 | Lactones–Unsaturated hydrocarbons                             | 11 |
| 199 | Fluorenes–Benzene and substituted derivatives                 | 11 |
| 200 | Saturated hydrocarbons–Phenols                                | 11 |
| 201 | Furans–Benzene and substituted derivatives                    | 11 |
| 202 | Phenol ethers–Organochlorides                                 | 11 |
| 203 | Lactones–Benzene and substituted derivatives                  | 11 |
| 204 | Organonitrogen compounds–Heteroaromatic compounds             | 11 |
| 205 | Organooxygen compounds–Organoiodides                          | 11 |

|     |                                                               |    |
|-----|---------------------------------------------------------------|----|
| 206 | Carboxylic acids and derivatives–Organochlorides              | 10 |
| 207 | Organooxygen compounds–Tetrahydrofurans                       | 10 |
| 208 | Carboximidic acids and derivatives–Alkyl halides              | 10 |
| 209 | Organoiodides–Benzene and substituted derivatives             | 10 |
| 210 | Phenols–Unsaturated hydrocarbons                              | 10 |
| 211 | Homogeneous other non-metal compounds–Organobromides          | 10 |
| 212 | Organochlorides–Unsaturated hydrocarbons                      | 10 |
| 213 | Alkyl halides–Organonitrogen compounds                        | 10 |
| 214 | Other non-metal organides–Saturated hydrocarbons              | 10 |
| 215 | Fatty Acyls–Vinyl halides                                     | 10 |
| 216 | Alkyl halides–Alkyl halides                                   | 10 |
| 217 | Thiols–Saturated hydrocarbons                                 | 10 |
| 218 | Phenol esters–Saturated hydrocarbons                          | 10 |
| 219 | Organooxygen compounds–Phenanthrenes and derivatives          | 10 |
| 220 | Pyrrolidines–Alkyl halides                                    | 10 |
| 221 | Phenanthrenes and derivatives–Saturated hydrocarbons          | 9  |
| 222 | Heteroaromatic compounds–Unsaturated hydrocarbons             | 9  |
| 223 | Benzene and substituted derivatives–Thioethers                | 9  |
| 224 | Saturated hydrocarbons–Tetrahydrofurans                       | 9  |
| 225 | Homogeneous other non-metal compounds–Phenol ethers           | 9  |
| 226 | Glycerolipids–Benzene and substituted derivatives             | 9  |
| 227 | Organic sulfonic acids and derivatives–Saturated hydrocarbons | 9  |
| 228 | Halohydrins–Benzene and substituted derivatives               | 9  |
| 229 | Saturated hydrocarbons–Organo-post-transition metal compounds | 9  |
| 230 | Organochlorides–Organonitrogen compounds                      | 9  |
| 231 | Homogeneous other non-metal compounds–Vinyl halides           | 9  |
| 232 | Keto acids and derivatives–Saturated hydrocarbons             | 9  |
| 233 | Oxathiolanes–Saturated hydrocarbons                           | 9  |
| 234 | Alkyl halides–Vinyl halides                                   | 9  |
| 235 | Organofluorides–Benzene and substituted derivatives           | 8  |
| 236 | Benzene and substituted derivatives–Other non-metal organides | 8  |
| 237 | Benzene and substituted derivatives–Organobromides            | 8  |
| 238 | Glycerolipids–Saturated hydrocarbons                          | 8  |
| 239 | Polycyclic hydrocarbons–Saturated hydrocarbons                | 8  |
| 240 | Tetrahydrofurans–Benzene and substituted derivatives          | 8  |
| 241 | Fatty Acyls–Allyl-type 1,3-dipolar organic compounds          | 8  |

|     |                                                                           |   |
|-----|---------------------------------------------------------------------------|---|
| 242 | Carboxylic acids and derivatives–Organonitrogen compounds                 | 8 |
| 243 | Piperidines–Benzene and substituted derivatives                           | 8 |
| 244 | Organooxygen compounds–Pyridines and derivatives                          | 8 |
| 245 | Azolidines–Benzene and substituted derivatives                            | 8 |
| 246 | Tetrahydrofurans–Organooxygen compounds                                   | 8 |
| 247 | Homogeneous other non-metal compounds–NA                                  | 8 |
| 248 | Oxolanes–Saturated hydrocarbons                                           | 8 |
| 249 | Allyl-type 1,3-dipolar organic compounds–Alkyl halides                    | 8 |
| 250 | Benzene and substituted derivatives–Organoiodides                         | 8 |
| 251 | Thioethers–Benzene and substituted derivatives                            | 8 |
| 252 | NA–Benzene and substituted derivatives                                    | 8 |
| 253 | Carboxylic acids and derivatives–Tetrahydrofurans                         | 8 |
| 254 | Phenol esters–Benzene and substituted derivatives                         | 7 |
| 255 | Prenol lipids–Organic oxoanionic compounds                                | 7 |
| 256 | Diarylheptanoids–Unsaturated hydrocarbons                                 | 7 |
| 257 | Glycerolipids–Organochlorides                                             | 7 |
| 258 | Thiophenols–Saturated hydrocarbons                                        | 7 |
| 259 | Glycerolipids–Carboxylic acids and derivatives                            | 7 |
| 260 | Glycerolipids–Alkyl halides                                               | 7 |
| 261 | Benzene and substituted derivatives–NA                                    | 7 |
| 262 | Benzene and substituted derivatives–Prenol lipids                         | 7 |
| 263 | Fatty Acyls–Organofluorides                                               | 7 |
| 264 | Benzene and substituted derivatives–Tetrahydrofurans                      | 7 |
| 265 | Carboxylic acids and derivatives–Heteroaromatic compounds                 | 7 |
| 266 | Acyl halides–Saturated hydrocarbons                                       | 7 |
| 267 | Azobenzenes–Saturated hydrocarbons                                        | 7 |
| 268 | Azoles–Benzene and substituted derivatives                                | 7 |
| 269 | Carboxylic acids and derivatives–NA                                       | 7 |
| 270 | Carboximidic acids and derivatives–Organonitrogen compounds               | 7 |
| 271 | Allyl-type 1,3-dipolar organic compounds–Organooxygen compounds           | 7 |
| 272 | Diarylheptanoids–Organochlorides                                          | 7 |
| 273 | Saturated hydrocarbons–Pyrrolidines                                       | 7 |
| 274 | Benzene and substituted derivatives–Homogeneous other non-metal compounds | 7 |
| 275 | Phenol ethers–Alkyl halides                                               | 7 |
| 276 | Oxazinanes–NA                                                             | 7 |
| 277 | Diarylheptanoids–Alkyl halides                                            | 7 |

|     |                                                                                |   |
|-----|--------------------------------------------------------------------------------|---|
| 278 | Dioxolanes–Saturated hydrocarbons                                              | 7 |
| 279 | Thiolanes–Carboxylic acids and derivatives                                     | 6 |
| 280 | NA–Alkyl halides                                                               | 6 |
| 281 | Organic sulfuric acids and derivatives–Saturated hydrocarbons                  | 6 |
| 282 | Organochlorides–Vinyl halides                                                  | 6 |
| 283 | Diarylheptanoids–Organooxygen compounds                                        | 6 |
| 284 | Thiolanes–Thioethers                                                           | 6 |
| 285 | Phenol ethers–Organooxygen compounds                                           | 6 |
| 286 | Pyrrolidines–NA                                                                | 6 |
| 287 | Organochlorides–Homogeneous other non-metal compounds                          | 6 |
| 288 | Organooxygen compounds–Anthracenes                                             | 6 |
| 289 | Organooxygen compounds–Tetralins                                               | 6 |
| 290 | Prenol lipids–Organonitrogen compounds                                         | 6 |
| 291 | Prenol lipids–Tetrahydrofurans                                                 | 6 |
| 292 | Organooxygen compounds–Organobromides                                          | 6 |
| 293 | Prenol lipids–Phenol esters                                                    | 6 |
| 294 | Saturated hydrocarbons–Thiols                                                  | 6 |
| 295 | NA–Carboxylic acids and derivatives                                            | 6 |
| 296 | Quinolines and derivatives–Organooxygen compounds                              | 6 |
| 297 | Organic phosphoric acids and derivatives–Homogeneous other non-metal compounds | 6 |
| 298 | Thioethers–Unsaturated hydrocarbons                                            | 6 |
| 299 | Hydroxy acids and derivatives–Organooxygen compounds                           | 6 |
| 300 | Unsaturated hydrocarbons–Organochlorides                                       | 6 |
| 301 | Organic sulfonic acids and derivatives–Unsaturated hydrocarbons                | 6 |
| 302 | Hydroxy acids and derivatives–Benzene and substituted derivatives              | 6 |
| 303 | Unsaturated hydrocarbons–Allyl-type 1,3-dipolar organic compounds              | 6 |
| 304 | Fatty Acyls–Tetrahydrofurans                                                   | 6 |
| 305 | Hydroxy acids and derivatives–Saturated hydrocarbons                           | 6 |
| 306 | Benzene and substituted derivatives–Phenol esters                              | 6 |
| 307 | Acyl halides–Organooxygen compounds                                            | 6 |
| 308 | Organo-post-transition metal compounds–Unsaturated hydrocarbons                | 6 |
| 309 | Carboximidic acids and derivatives–Organochlorides                             | 6 |
| 310 | Naphthalenes–Alkyl halides                                                     | 6 |
| 311 | Organooxygen compounds–Thioethers                                              | 6 |
| 312 | Organochlorides–Carboxylic acids and derivatives                               | 6 |
| 313 | Saturated hydrocarbons–Prenol lipids                                           | 5 |

|     |                                                                                |   |
|-----|--------------------------------------------------------------------------------|---|
| 314 | Alkyl halides–Carboxylic acids and derivatives                                 | 5 |
| 315 | Homogeneous other non-metal compounds–Pyridines and derivatives                | 5 |
| 316 | Stilbenes–Benzene and substituted derivatives                                  | 5 |
| 317 | Unsaturated hydrocarbons–Alkyl halides                                         | 5 |
| 318 | Fatty Acyls–Fatty Acyls                                                        | 5 |
| 319 | Carboxylic acids and derivatives–Dioxanes                                      | 5 |
| 320 | Homogeneous other non-metal compounds–Naphthalenes                             | 5 |
| 321 | Organonitrogen compounds–Thiolanes                                             | 5 |
| 322 | Unsaturated hydrocarbons–Organonitrogen compounds                              | 5 |
| 323 | Glycerolipids–Organofluorides                                                  | 5 |
| 324 | Organochlorides–Allyl-type 1,3-dipolar organic compounds                       | 5 |
| 325 | Benzene and substituted derivatives–Carboximidic acids and derivatives         | 5 |
| 326 | Saturated hydrocarbons–Lactams                                                 | 5 |
| 327 | Benzene and substituted derivatives–Organic oxoanionic compounds               | 5 |
| 328 | Prenol lipids–Allyl-type 1,3-dipolar organic compounds                         | 5 |
| 329 | Oxolanes–Unsaturated hydrocarbons                                              | 5 |
| 330 | Homogeneous other non-metal compounds–Allyl-type 1,3-dipolar organic compounds | 5 |
| 331 | Organic phosphoric acids and derivatives–Organochlorides                       | 5 |
| 332 | Pyrrolidines–Carboxylic acids and derivatives                                  | 5 |
| 333 | Prenol lipids–Fatty Acyls                                                      | 5 |
| 334 | Fluorenes–Saturated hydrocarbons                                               | 5 |
| 335 | Benzofurans–Saturated hydrocarbons                                             | 5 |
| 336 | Saturated hydrocarbons–Vinyl halides                                           | 5 |
| 337 | Azolidines–NA                                                                  | 5 |
| 338 | Oxazinanes–Carboxylic acids and derivatives                                    | 5 |
| 339 | Organoiodides–Saturated hydrocarbons                                           | 5 |
| 340 | Prenol lipids–Phenols                                                          | 5 |
| 341 | Organic phosphoric acids and derivatives–Phenol esters                         | 4 |
| 342 | Organic phosphoric acids and derivatives–Dioxanes                              | 4 |
| 343 | Benzene and substituted derivatives–Aryl halides                               | 4 |
| 344 | Acyl halides–Carboxylic acids and derivatives                                  | 4 |
| 345 | Organofluorides–Unsaturated hydrocarbons                                       | 4 |
| 346 | Phenols–Organochlorides                                                        | 4 |
| 347 | Alkyl halides–Organoiodides                                                    | 4 |
| 348 | Phenols–Naphthalenes                                                           | 4 |
| 349 | Alkyl halides–Organo-post-transition metal compounds                           | 4 |

|     |                                                                            |   |
|-----|----------------------------------------------------------------------------|---|
| 350 | Saturated hydrocarbons–Dioxanes                                            | 4 |
| 351 | Acyl halides–Unsaturated hydrocarbons                                      | 4 |
| 352 | Saturated hydrocarbons–Other non-metal organides                           | 4 |
| 353 | Sulfonyls–Benzene and substituted derivatives                              | 4 |
| 354 | Allyl-type 1,3-dipolar organic compounds–Organochlorides                   | 4 |
| 355 | Vinyl halides–Benzene and substituted derivatives                          | 4 |
| 356 | Prenol lipids–Aryl halides                                                 | 4 |
| 357 | Saturated hydrocarbons–Polycyclic hydrocarbons                             | 4 |
| 358 | Vinyl halides–Organochlorides                                              | 4 |
| 359 | Thiolanes–Thiols                                                           | 4 |
| 360 | Organooxygen compounds–Polycyclic hydrocarbons                             | 4 |
| 361 | Tetrahydrofurans–Alkyl halides                                             | 4 |
| 362 | Saturated hydrocarbons–Oxazinanones                                        | 4 |
| 363 | Saturated hydrocarbons–Thioethers                                          | 4 |
| 364 | Saturated hydrocarbons–Heteroaromatic compounds                            | 4 |
| 365 | Pyridines and derivatives–Unsaturated hydrocarbons                         | 4 |
| 366 | Alkyl halides–Allyl-type 1,3-dipolar organic compounds                     | 4 |
| 367 | Pyridines and derivatives–Organooxygen compounds                           | 4 |
| 368 | Polycyclic hydrocarbons–Unsaturated hydrocarbons                           | 4 |
| 369 | Alkyl halides–Homogeneous other non-metal compounds                        | 4 |
| 370 | Dioxanes–Unsaturated hydrocarbons                                          | 4 |
| 371 | Dioxolanes–Unsaturated hydrocarbons                                        | 4 |
| 372 | Naphthalenes–Carboxylic acids and derivatives                              | 4 |
| 373 | Naphthalenes–Organonitrogen compounds                                      | 4 |
| 374 | Organonitrogen compounds–Thiols                                            | 4 |
| 375 | Organonitrogen compounds–Phenol esters                                     | 4 |
| 376 | Thiolanes–Heteroaromatic compounds                                         | 4 |
| 377 | Benzene and substituted derivatives–Organo-post-transition metal compounds | 4 |
| 378 | Organonitrogen compounds–Other non-metal organides                         | 4 |
| 379 | Organonitrogen compounds–Dioxanes                                          | 4 |
| 380 | Diarylheptanoids–Carboxylic acids and derivatives                          | 4 |
| 381 | Carboxylic acids and derivatives–Homogeneous other non-metal compounds     | 4 |
| 382 | Thiols–Organooxygen compounds                                              | 4 |
| 383 | Organic carbonic acids and derivatives–Organochlorides                     | 4 |
| 384 | Organic carbonic acids and derivatives–Organonitrogen compounds            | 4 |
| 385 | Organic oxides–Unsaturated hydrocarbons                                    | 4 |

|     |                                                                           |   |
|-----|---------------------------------------------------------------------------|---|
| 386 | Benzene and substituted derivatives–Thiols                                | 4 |
| 387 | Glycerolipids–Fatty Acyls                                                 | 4 |
| 388 | Organic carbonic acids and derivatives–Carboxylic acids and derivatives   | 4 |
| 389 | Organic oxides–Saturated hydrocarbons                                     | 4 |
| 390 | Unsaturated hydrocarbons–Prenol lipids                                    | 4 |
| 391 | Organooxygen compounds–Thiols                                             | 4 |
| 392 | Carboxylic acids and derivatives–Allyl-type 1,3-dipolar organic compounds | 4 |
| 393 | Dioxanes–Benzene and substituted derivatives                              | 4 |
| 394 | Sulfoxides–Carboxylic acids and derivatives                               | 4 |
| 395 | Carboxylic acids and derivatives–Other non-metal organides                | 4 |
| 396 | Organooxygen compounds–Other non-metal organides                          | 4 |
| 397 | Sulfoxides–Acyclic allenes                                                | 4 |
| 398 | Fatty Acyls–Homogeneous other non-metal compounds                         | 4 |
| 399 | Fatty Acyls–Phenol ethers                                                 | 4 |
| 400 | Organonitrogen compounds–Allyl-type 1,3-dipolar organic compounds         | 4 |
| 401 | Organonitrogen compounds–Phenols                                          | 4 |
| 402 | Organooxygen compounds–Prenol lipids                                      | 4 |
| 403 | Tetralins–Unsaturated hydrocarbons                                        | 4 |
| 404 | Organochlorides–Organo-post-transition metal compounds                    | 4 |
| 405 | Glycerolipids–Heteroaromatic compounds                                    | 4 |
| 406 | Organofluorides–Organofluorides                                           | 4 |
| 407 | Organic carbonic acids and derivatives–Alkyl halides                      | 4 |
| 408 | Organooxygen compounds–Organometalloid compounds                          | 4 |
| 409 | Organooxygen compounds–Phenols                                            | 4 |
| 410 | Alkyl halides–Tetrahydrofurans                                            | 3 |
| 411 | Organonitrogen compounds–Organobromides                                   | 3 |
| 412 | Carboxylic acids and derivatives–Organofluorides                          | 3 |
| 413 | Benzene and substituted derivatives–Phenol ethers                         | 3 |
| 414 | Quinolines and derivatives–Alkyl halides                                  | 3 |
| 415 | Organofluorides–Carboxylic acids and derivatives                          | 3 |
| 416 | Prenol lipids–Phenol ethers                                               | 3 |
| 417 | Carboximidic acids and derivatives–Tetrahydrofurans                       | 3 |
| 418 | Alkyl halides–Organofluorides                                             | 3 |
| 419 | Homogeneous other non-metal compounds–Heteroaromatic compounds            | 3 |
| 420 | Organofluorides–Alkyl halides                                             | 3 |
| 421 | Organo-post-transition metal compounds–Alkyl halides                      | 3 |

|     |                                                                  |   |
|-----|------------------------------------------------------------------|---|
| 422 | Other non-metal organides–Organooxygen compounds                 | 3 |
| 423 | Phenols–Organooxygen compounds                                   | 3 |
| 424 | Homogeneous other non-metal compounds–Quinolines and derivatives | 3 |
| 425 | Pyrrolidines–Tetrahydrofurans                                    | 3 |
| 426 | Piperidines–Carboxylic acids and derivatives                     | 3 |
| 427 | Prenol lipids–Vinyl halides                                      | 3 |
| 428 | Vinyl halides–Unsaturated hydrocarbons                           | 3 |
| 429 | Vinyl halides–Homogeneous other non-metal compounds              | 3 |
| 430 | Vinyl halides–Alkyl halides                                      | 3 |
| 431 | Vinyl halides–Vinyl halides                                      | 3 |
| 432 | Azolidines–Carboxylic acids and derivatives                      | 3 |
| 433 | Heteroaromatic compounds–Benzene and substituted derivatives     | 3 |
| 434 | Vinyl halides–Saturated hydrocarbons                             | 3 |
| 435 | Homogeneous other non-metal compounds–Thiols                     | 3 |
| 436 | Hydroxy acids and derivatives–Unsaturated hydrocarbons           | 3 |
| 437 | Organoiodides–Alkyl halides                                      | 3 |
| 438 | Organic metal salts–Benzene and substituted derivatives          | 3 |
| 439 | Saturated hydrocarbons–Halohydrins                               | 3 |
| 440 | Hydroxy acids and derivatives–Organochlorides                    | 3 |
| 441 | Allyl-type 1,3-dipolar organic compounds–Organoiodides           | 3 |
| 442 | Acyl halides–Organochlorides                                     | 3 |
| 443 | Phenanthrenes and derivatives–Organooxygen compounds             | 3 |
| 444 | Phenols–Alkyl halides                                            | 3 |
| 445 | Oxathiolanes–Unsaturated hydrocarbons                            | 3 |
| 446 | Acyl halides–Organonitrogen compounds                            | 3 |
| 447 | Hydroxy acids and derivatives–Organonitrogen compounds           | 3 |
| 448 | Glycerolipids–Tetrahydrofurans                                   | 3 |
| 449 | Sulfoxides–Alkyl halides                                         | 3 |
| 450 | Unsaturated hydrocarbons–Homogeneous other non-metal compounds   | 3 |
| 451 | Saturated hydrocarbons–Carboximide acids and derivatives         | 3 |
| 452 | Benzofurans–Benzene and substituted derivatives                  | 3 |
| 453 | Thiolanes–NA                                                     | 3 |
| 454 | Saturated hydrocarbons–Thiolanes                                 | 3 |
| 455 | NA–Organochlorides                                               | 3 |
| 456 | Glycerolipids–Vinyl halides                                      | 3 |
| 457 | Glycerolipids–Allyl-type 1,3-dipolar organic compounds           | 3 |

|     |                                                                                |   |
|-----|--------------------------------------------------------------------------------|---|
| 458 | Organic carbonic acids and derivatives–Unsaturated hydrocarbons                | 3 |
| 459 | Saturated hydrocarbons–Sulfoxides                                              | 3 |
| 460 | Benzene and substituted derivatives–Pyridines and derivatives                  | 3 |
| 461 | Thiolanes–Polycyclic hydrocarbons                                              | 3 |
| 462 | Organooxygen compounds–NA                                                      | 3 |
| 463 | Organic phosphoric acids and derivatives–Organonitrogen compounds              | 3 |
| 464 | Fatty Acyls–Organobromides                                                     | 3 |
| 465 | Diarylheptanoids–Vinyl halides                                                 | 3 |
| 466 | Depsidones and depsidones–Organooxygen compounds                               | 3 |
| 467 | Hydroxy acids and derivatives–Carboxylic acids and derivatives                 | 3 |
| 468 | Thiolanes–Alkyl halides                                                        | 3 |
| 469 | Diazinanes–Benzene and substituted derivatives                                 | 3 |
| 470 | Indenes and isoindenes–Saturated hydrocarbons                                  | 3 |
| 471 | Homogeneous other non-metal compounds–Organiodides                             | 3 |
| 472 | Saturated hydrocarbons–Naphthalenes                                            | 3 |
| 473 | Benzene and substituted derivatives–Organometalloid compounds                  | 3 |
| 474 | Dioxolanes–Benzene and substituted derivatives                                 | 2 |
| 475 | Heteroaromatic compounds–NA                                                    | 2 |
| 476 | Naphthalenes–Pyridines and derivatives                                         | 2 |
| 477 | Naphthalenes–Allyl-type 1,3-dipolar organic compounds                          | 2 |
| 478 | Dioxanes–Organooxygen compounds                                                | 2 |
| 479 | Naphthalenes–Organochlorides                                                   | 2 |
| 480 | Oxathiolanes–Benzene and substituted derivatives                               | 2 |
| 481 | Piperidines–Alkyl halides                                                      | 2 |
| 482 | Fatty Acyls–Heteroaromatic compounds                                           | 2 |
| 483 | Homogeneous other non-metal compounds–Piperidines                              | 2 |
| 484 | Homogeneous other non-metal compounds–Organic phosphonic acids and derivatives | 2 |
| 485 | Homogeneous other non-metal compounds–Lactones                                 | 2 |
| 486 | Organonitrogen compounds–Organometalloid compounds                             | 2 |
| 487 | Acyl halides–Benzene and substituted derivatives                               | 2 |
| 488 | NA–Pyrrolidines                                                                | 2 |
| 489 | NA–Sulfoxides                                                                  | 2 |
| 490 | Lactams–Prenol lipids                                                          | 2 |
| 491 | Thiols–Carboxylic acids and derivatives                                        | 2 |
| 492 | Homogeneous other non-metal compounds–Organometalloid compounds                | 2 |
| 493 | Homogeneous other non-metal compounds–Organic oxides                           | 2 |

|     |                                                                            |   |
|-----|----------------------------------------------------------------------------|---|
| 494 | Acyl halides–Alkyl halides                                                 | 2 |
| 495 | Isoquinolines and derivatives–Unsaturated hydrocarbons                     | 2 |
| 496 | Quinolines and derivatives–Organochlorides                                 | 2 |
| 497 | Hydroxy acids and derivatives–Alkyl halides                                | 2 |
| 498 | Pyridines and derivatives–Homogeneous other non-metal compounds            | 2 |
| 499 | Lactones–Alkyl halides                                                     | 2 |
| 500 | Allyl-type 1,3-dipolar organic compounds–Other non-metal organides         | 2 |
| 501 | Thiols–Unsaturated hydrocarbons                                            | 2 |
| 502 | Allyl-type 1,3-dipolar organic compounds–Organobromides                    | 2 |
| 503 | Phenanthrenes and derivatives–Unsaturated hydrocarbons                     | 2 |
| 504 | Halohydrins–NA                                                             | 2 |
| 505 | Pyridines and derivatives–Allyl-type 1,3-dipolar organic compounds         | 2 |
| 506 | Pyrroles–Benzene and substituted derivatives                               | 2 |
| 507 | Alkyl halides–Dioxanes                                                     | 2 |
| 508 | Unsaturated hydrocarbons–Pyrrolidines                                      | 2 |
| 509 | NA–Thiolanes                                                               | 2 |
| 510 | Saturated hydrocarbons–Phenol ethers                                       | 2 |
| 511 | Pyridines and derivatives–Dioxanes                                         | 2 |
| 512 | Lactones–Carboxylic acids and derivatives                                  | 2 |
| 513 | Tetrahydrofurans–Carboxylic acids and derivatives                          | 2 |
| 514 | Sulfoxides–NA                                                              | 2 |
| 515 | Tetralins–Saturated hydrocarbons                                           | 2 |
| 516 | Homogeneous other non-metal compounds–Oxanes                               | 2 |
| 517 | Organic phosphoric acids and derivatives–Other non-metal organides         | 2 |
| 518 | Organochlorides–Organobromides                                             | 2 |
| 519 | Benzene and substituted derivatives–Phenols                                | 2 |
| 520 | Phenol ethers–Vinyl halides                                                | 2 |
| 521 | Organic sulfonic acids and derivatives–Benzene and substituted derivatives | 2 |
| 522 | Organic sulfuric acids and derivatives–Benzene and substituted derivatives | 2 |
| 523 | Organic phosphoric acids and derivatives–Phenols                           | 2 |
| 524 | Benzofurans–Organooxygen compounds                                         | 2 |
| 525 | Thiophenols–Benzene and substituted derivatives                            | 2 |
| 526 | Organic phosphoric acids and derivatives–Organometalloid compounds         | 2 |
| 527 | NA–Organonitrogen compounds                                                | 2 |
| 528 | Phenol ethers–Prenol lipids                                                | 2 |
| 529 | Phenol esters–Unsaturated hydrocarbons                                     | 2 |

|     |                                                                              |   |
|-----|------------------------------------------------------------------------------|---|
| 530 | Thiolanes–Prenol lipids                                                      | 2 |
| 531 | Thiolanes–Organochlorides                                                    | 2 |
| 532 | Benzene and substituted derivatives–Thiolanes                                | 2 |
| 533 | Organometalloid compounds–Homogeneous other non-metal compounds              | 2 |
| 534 | Benzene and substituted derivatives–Organofluorides                          | 2 |
| 535 | Diarylheptanoids–Organonitrogen compounds                                    | 2 |
| 536 | Saturated hydrocarbons–Dioxolanes                                            | 2 |
| 537 | Organochlorides–Organoiodides                                                | 2 |
| 538 | Keto acids and derivatives–Unsaturated hydrocarbons                          | 2 |
| 539 | Piperidines–NA                                                               | 2 |
| 540 | Glycerolipids–Phenol ethers                                                  | 2 |
| 541 | Other non-metal organides–Benzene and substituted derivatives                | 2 |
| 542 | Glycerolipids–Unsaturated hydrocarbons                                       | 2 |
| 543 | Organobromides–Homogeneous other non-metal compounds                         | 2 |
| 544 | Organonitrogen compounds–Tetrahydrofurans                                    | 2 |
| 545 | Fluorenes–Organonitrogen compounds                                           | 2 |
| 546 | Prenol lipids–Organobromides                                                 | 2 |
| 547 | Pyrrolidines–Prenol lipids                                                   | 2 |
| 548 | Thiols–Benzene and substituted derivatives                                   | 2 |
| 549 | Organic oxides–Benzene and substituted derivatives                           | 2 |
| 550 | Oxazinanones–Acyclic allenes                                                 | 2 |
| 551 | Organonitrogen compounds–Pyridines and derivatives                           | 2 |
| 552 | Carboxylic acids and derivatives–Vinyl halides                               | 2 |
| 553 | Carboxylic acids and derivatives–Pyridines and derivatives                   | 2 |
| 554 | Phenols–Phenanthrenes and derivatives                                        | 2 |
| 555 | Homogeneous other non-metal compounds–Organo-post-transition metal compounds | 2 |
| 556 | Prenol lipids–Organometalloid compounds                                      | 2 |
| 557 | Homogeneous other non-metal compounds–Tetrahydrofurans                       | 2 |
| 558 | Organochlorides–Tetrahydrofurans                                             | 2 |
| 559 | Homogeneous other non-metal compounds–Indoles and derivatives                | 2 |
| 560 | Carboxylic acids and derivatives–Organoiodides                               | 2 |
| 561 | Carboxylic acids and derivatives–Organobromides                              | 2 |
| 562 | Fluorenes–Organooxygen compounds                                             | 2 |
| 563 | Carboximide acids and derivatives–Fatty Acyls                                | 2 |
| 564 | Organonitrogen compounds–Homogeneous other non-metal compounds               | 2 |
| 565 | Pyrrolidines–Homogeneous other non-metal compounds                           | 2 |

|     |                                                                                |   |
|-----|--------------------------------------------------------------------------------|---|
| 566 | Organonitrogen compounds–Organoiodides                                         | 2 |
| 567 | Dioxanes–Alkyl halides                                                         | 2 |
| 568 | Homogeneous other non-metal compounds–Organic phosphoric acids and derivatives | 1 |
| 569 | Piperidines–Homogeneous other non-metal compounds                              | 1 |
| 570 | Homogeneous other non-metal compounds–Tetralins                                | 1 |
| 571 | Hydroxy acids and derivatives–Homogeneous other non-metal compounds            | 1 |
| 572 | Organobromides–Carboxylic acids and derivatives                                | 1 |
| 573 | Organobromides–Organochlorides                                                 | 1 |
| 574 | Homogeneous other non-metal compounds–Organic oxoanionic compounds             | 1 |
| 575 | Organobromides–Organonitrogen compounds                                        | 1 |
| 576 | Hydroxy acids and derivatives–Allyl-type 1,3-dipolar organic compounds         | 1 |
| 577 | Homogeneous other non-metal compounds–Homogeneous other non-metal compounds    | 1 |
| 578 | Homogeneous other non-metal compounds–Indanes                                  | 1 |
| 579 | Homogeneous other non-metal compounds–Homogeneous halogens                     | 1 |
| 580 | Homogeneous other non-metal compounds–Thioethers                               | 1 |
| 581 | Homogeneous other non-metal compounds–Homogeneous transition metal compounds   | 1 |
| 582 | Homogeneous other non-metal compounds–Sulfoxides                               | 1 |
| 583 | Pyrroles–Saturated hydrocarbons                                                | 1 |
| 584 | Thiolanes–Indenes and isoindenes                                               | 1 |
| 585 | Homogeneous other non-metal compounds–Epoxides                                 | 1 |
| 586 | Homogeneous other non-metal compounds–Dioxanes                                 | 1 |
| 587 | Organooxygen compounds–Indenes and isoindenes                                  | 1 |
| 588 | Sulfonyls–Acyclic allenes                                                      | 1 |
| 589 | Organooxygen compounds–Organic sulfuric acids and derivatives                  | 1 |
| 590 | Benzene and substituted derivatives–Oxacyclic compounds                        | 1 |
| 591 | Phenols–Allyl-type 1,3-dipolar organic compounds                               | 1 |
| 592 | Tetralins–Benzene and substituted derivatives                                  | 1 |
| 593 | Tetralins–NA                                                                   | 1 |
| 594 | Thiolanes–Other non-metal organides                                            | 1 |
| 595 | Thiolanes–Dioxanes                                                             | 1 |
| 596 | Sulfoxides–Homogeneous other non-metal compounds                               | 1 |
| 597 | Sulfoxides–Heteroaromatic compounds                                            | 1 |
| 598 | Sulfoxides–Organo-post-transition metal compounds                              | 1 |
| 599 | Sulfoxides–Pyrrolidines                                                        | 1 |
| 600 | Sulfoxides–Allyl-type 1,3-dipolar organic compounds                            | 1 |
| 601 | Sulfoxides–Tetrahydrofurans                                                    | 1 |

|     |                                                                              |   |
|-----|------------------------------------------------------------------------------|---|
| 602 | Sulfoxides–Organoiodides                                                     | 1 |
| 603 | Sulfoxides–Organochlorides                                                   | 1 |
| 604 | Thiolanes–Organonitrogen compounds                                           | 1 |
| 605 | Sulfoxides–Organonitrogen compounds                                          | 1 |
| 606 | Diazinanes–NA                                                                | 1 |
| 607 | Sulfoxides–Dioxanes                                                          | 1 |
| 608 | Thiolanes–Homogeneous other non-metal compounds                              | 1 |
| 609 | Thiolanes–Thiolanes                                                          | 1 |
| 610 | Thiolanes–Tetralins                                                          | 1 |
| 611 | Thiolanes–Pyridines and derivatives                                          | 1 |
| 612 | Thiolanes–Oxanes                                                             | 1 |
| 613 | Thiolanes–Vinyl halides                                                      | 1 |
| 614 | Thiolanes–Tetrahydrofurans                                                   | 1 |
| 615 | Thiolanes–Naphthalenes                                                       | 1 |
| 616 | Organooxygen compounds–Thiolanes                                             | 1 |
| 617 | Organo-post-transition metal compounds–Organochlorides                       | 1 |
| 618 | Homogeneous other non-metal compounds–Organic disulfides                     | 1 |
| 619 | Homogeneous other non-metal compounds–Halohydrins                            | 1 |
| 620 | Homogeneous other non-metal compounds–Organophosphinic acids and derivatives | 1 |
| 621 | Homogeneous other non-metal compounds–Dioxolanes                             | 1 |
| 622 | Pyridines and derivatives–NA                                                 | 1 |
| 623 | Pyridines and derivatives–Carboximidic acids and derivatives                 | 1 |
| 624 | Quinolines and derivatives–NA                                                | 1 |
| 625 | Homogeneous other non-metal compounds–Other non-metal organides              | 1 |
| 626 | Quinolines and derivatives–Carboxylic acids and derivatives                  | 1 |
| 627 | Quinolines and derivatives–Organonitrogen compounds                          | 1 |
| 628 | Quinolines and derivatives–Organobromides                                    | 1 |
| 629 | Quinolines and derivatives–Organoiodides                                     | 1 |
| 630 | Homogeneous other non-metal compounds–Keto acids and derivatives             | 1 |
| 631 | Homogeneous other non-metal compounds–Phenanthrenes and derivatives          | 1 |
| 632 | Organometalloid compounds–Unsaturated hydrocarbons                           | 1 |
| 633 | Organometalloid compounds–Benzene and substituted derivatives                | 1 |
| 634 | Homogeneous other non-metal compounds–Pyrenes                                | 1 |
| 635 | Prenol lipids–Dioxanes                                                       | 1 |
| 636 | Prenol lipids–Pyrrolidines                                                   | 1 |
| 637 | Homogeneous other non-metal compounds–Benzothiophenes                        | 1 |

|     |                                                                          |   |
|-----|--------------------------------------------------------------------------|---|
| 638 | Prenol lipids–Other non-metal organides                                  | 1 |
| 639 | Prenol lipids–Organic carbonic acids and derivatives                     | 1 |
| 640 | Homogeneous other non-metal compounds–Anthracenes                        | 1 |
| 641 | Homogeneous other non-metal compounds–Phenol esters                      | 1 |
| 642 | Homogeneous other non-metal compounds–Carboximidic acids and derivatives | 1 |
| 643 | Homogeneous other non-metal compounds–Glycerolipids                      | 1 |
| 644 | Prenol lipids–Organic phosphoric acids and derivatives                   | 1 |
| 645 | Prenol lipids–Trialkylphosphites                                         | 1 |
| 646 | Prenol lipids–Sulfoxides                                                 | 1 |
| 647 | Prenol lipids–Thiophenes                                                 | 1 |
| 648 | Organic metal salts–Unsaturated hydrocarbons                             | 1 |
| 649 | Homogeneous other non-metal compounds–Pyrrolidines                       | 1 |
| 650 | NA–Pyridines and derivatives                                             | 1 |
| 651 | Benzene and substituted derivatives–Thiophenes                           | 1 |
| 652 | Carboximidic acids and derivatives–Pyridines and derivatives             | 1 |
| 653 | Organonitrogen compounds–Naphthalenes                                    | 1 |
| 654 | Phenol ethers–Phenol ethers                                              | 1 |
| 655 | Organonitrogen compounds–Organofluorides                                 | 1 |
| 656 | Organonitrogen compounds–Phenol ethers                                   | 1 |
| 657 | Organonitrogen compounds–Carboximidic acids and derivatives              | 1 |
| 658 | Organonitrogen compounds–Organo-post-transition metal compounds          | 1 |
| 659 | Organonitrogen compounds–Oxacyclic compounds                             | 1 |
| 660 | Carboxylic acids and derivatives–Organo-post-transition metal compounds  | 1 |
| 661 | Carboximidic acids and derivatives–Homogeneous other non-metal compounds | 1 |
| 662 | Carboximidic acids and derivatives–Phenols                               | 1 |
| 663 | Depsidones and depsidones–Organonitrogen compounds                       | 1 |
| 664 | Carboximidic acids and derivatives–Naphthalenes                          | 1 |
| 665 | Carboximidic acids and derivatives–Heteroaromatic compounds              | 1 |
| 666 | Carboximidic acids and derivatives–Vinyl halides                         | 1 |
| 667 | Carboximidic acids and derivatives–Dioxanes                              | 1 |
| 668 | Quinolines and derivatives–Phenol ethers                                 | 1 |
| 669 | Oxazinanes–Heteroaromatic compounds                                      | 1 |
| 670 | Oxazinanes–Tetrahydrofurans                                              | 1 |
| 671 | Oxazinanes–Fatty Acyls                                                   | 1 |
| 672 | Oxazinanes–Dioxanes                                                      | 1 |
| 673 | Depsidones and depsidones–Carboxylic acids and derivatives               | 1 |

|     |                                                                |   |
|-----|----------------------------------------------------------------|---|
| 674 | Depsides and depsidones–Organochlorides                        | 1 |
| 675 | Dihydrofurans–Saturated hydrocarbons                           | 1 |
| 676 | Phenol ethers–Organoiodides                                    | 1 |
| 677 | Diarylheptanoids–Allyl-type 1,3-dipolar organic compounds      | 1 |
| 678 | Diarylheptanoids–Organic carbonic acids and derivatives        | 1 |
| 679 | Diarylheptanoids–Other non-metal organides                     | 1 |
| 680 | Diarylheptanoids–Phenol ethers                                 | 1 |
| 681 | Benzene and substituted derivatives–Lactams                    | 1 |
| 682 | Benzene and substituted derivatives–Pyrrolidines               | 1 |
| 683 | Phenol ethers–Other non-metal organides                        | 1 |
| 684 | Phenol ethers–Allyl-type 1,3-dipolar organic compounds         | 1 |
| 685 | Phenol ethers–Dioxanes                                         | 1 |
| 686 | Phenol ethers–Organobromides                                   | 1 |
| 687 | Depsides and depsidones–Fatty Acyls                            | 1 |
| 688 | Phenol ethers–Organonitrogen compounds                         | 1 |
| 689 | Phenol ethers–Carboxylic acids and derivatives                 | 1 |
| 690 | Benzene and substituted derivatives–Naphthalenes               | 1 |
| 691 | Phenol esters–Fatty Acyls                                      | 1 |
| 692 | Phenol esters–Organochlorides                                  | 1 |
| 693 | Phenol esters–Organonitrogen compounds                         | 1 |
| 694 | Phenol esters–Carboxylic acids and derivatives                 | 1 |
| 695 | Phenol esters–Organooxygen compounds                           | 1 |
| 696 | Depsides and depsidones–Unsaturated hydrocarbons               | 1 |
| 697 | Oxolanes–Benzene and substituted derivatives                   | 1 |
| 698 | Dihydrofurans–Benzene and substituted derivatives              | 1 |
| 699 | Keto acids and derivatives–Benzene and substituted derivatives | 1 |
| 700 | Oxathianes–Saturated hydrocarbons                              | 1 |
| 701 | Fatty Acyls–Other non-metal organides                          | 1 |
| 702 | Fatty Acyls–Dioxanes                                           | 1 |
| 703 | Unsaturated hydrocarbons–Heteroaromatic compounds              | 1 |
| 704 | Unsaturated hydrocarbons–Organobromides                        | 1 |
| 705 | Aziridines–Saturated hydrocarbons                              | 1 |
| 706 | Aziridines–Benzene and substituted derivatives                 | 1 |
| 707 | Thiols–Alkyl halides                                           | 1 |
| 708 | Thiols–Organochlorides                                         | 1 |
| 709 | Thiols–Organonitrogen compounds                                | 1 |

|     |                                                                               |   |
|-----|-------------------------------------------------------------------------------|---|
| 710 | Oxathianes–Benzene and substituted derivatives                                | 1 |
| 711 | Fatty Acyls–Halohydrins                                                       | 1 |
| 712 | Oxathianes–Unsaturated hydrocarbons                                           | 1 |
| 713 | Dioxanes–Phenols                                                              | 1 |
| 714 | Dioxanes–Allyl-type 1,3-dipolar organic compounds                             | 1 |
| 715 | Dioxanes–Organoiodides                                                        | 1 |
| 716 | Dioxanes–Organonitrogen compounds                                             | 1 |
| 717 | Carboxylic acids and derivatives–Phenol ethers                                | 1 |
| 718 | Organic carbonic acids and derivatives–Organo-post-transition metal compounds | 1 |
| 719 | Organic carbonic acids and derivatives–Organoiodides                          | 1 |
| 720 | Organic carbonic acids and derivatives–Homogeneous other non-metal compounds  | 1 |
| 721 | Fatty Acyls–Organoiodides                                                     | 1 |
| 722 | Fatty Acyls–Epoxides                                                          | 1 |
| 723 | Pyrrolidines–Heteroaromatic compounds                                         | 1 |
| 724 | Halohydrins–Dioxanes                                                          | 1 |
| 725 | Pyrrolidines–Organo-post-transition metal compounds                           | 1 |
| 726 | Pyrrolidines–Allyl-type 1,3-dipolar organic compounds                         | 1 |
| 727 | Pyrrolidines–Other non-metal organides                                        | 1 |
| 728 | Pyrrolidines–Fatty Acyls                                                      | 1 |
| 729 | Pyrrolidines–Polycyclic hydrocarbons                                          | 1 |
| 730 | Pyrrolidines–Dioxanes                                                         | 1 |
| 731 | Pyrrolidines–Vinyl halides                                                    | 1 |
| 732 | Halohydrins–Allyl-type 1,3-dipolar organic compounds                          | 1 |
| 733 | Halohydrins–Organooxygen compounds                                            | 1 |
| 734 | Piperidines–Tetrahydrofurans                                                  | 1 |
| 735 | Fatty Acyls–Oxanes                                                            | 1 |
| 736 | Piperidines–Organonitrogen compounds                                          | 1 |
| 737 | Azolidines–Dioxanes                                                           | 1 |
| 738 | Organooxygen compounds–Phenol ethers                                          | 1 |
| 739 | Oxathiolanes–NA                                                               | 1 |
| 740 | Unsaturated hydrocarbons–Oxazinanes                                           | 1 |
| 741 | Unsaturated hydrocarbons–Carboximide acids and derivatives                    | 1 |
| 742 | Fatty Acyls–Sulfoxides                                                        | 1 |
| 743 | Fatty Acyls–Organo-post-transition metal compounds                            | 1 |
| 744 | Fatty Acyls–Pyridines and derivatives                                         | 1 |
| 745 | Organochlorides–Other non-metal organides                                     | 1 |

|     |                                                                                   |   |
|-----|-----------------------------------------------------------------------------------|---|
| 746 | Lactones–Dioxanes                                                                 | 1 |
| 747 | Benzene and substituted derivatives–Epoxides                                      | 1 |
| 748 | Lactams–Polycyclic hydrocarbons                                                   | 1 |
| 749 | Alkyl halides–Fatty Acyls                                                         | 1 |
| 750 | Alkyl halides–Unsaturated hydrocarbons                                            | 1 |
| 751 | Allyl-type 1,3-dipolar organic compounds–Homogeneous other non-metal compounds    | 1 |
| 752 | Allyl-type 1,3-dipolar organic compounds–Organonitrogen compounds                 | 1 |
| 753 | Isoquinolines and derivatives–Benzene and substituted derivatives                 | 1 |
| 754 | Indenes and isoindenes–Benzene and substituted derivatives                        | 1 |
| 755 | Indenes and isoindenes–Unsaturated hydrocarbons                                   | 1 |
| 756 | Lactams–Alkyl halides                                                             | 1 |
| 757 | Lactams–Organochlorides                                                           | 1 |
| 758 | Lactams–Organooxygen compounds                                                    | 1 |
| 759 | Alkyl halides–Phenols                                                             | 1 |
| 760 | Lactams–NA                                                                        | 1 |
| 761 | Lactams–Dioxanes                                                                  | 1 |
| 762 | Organofluorides–Allyl-type 1,3-dipolar organic compounds                          | 1 |
| 763 | Organofluorides–Dioxanes                                                          | 1 |
| 764 | Lactones–Tetrahydrofurans                                                         | 1 |
| 765 | Fatty Acyls–Prenol lipids                                                         | 1 |
| 766 | Saturated hydrocarbons–Oxanes                                                     | 1 |
| 767 | Saturated hydrocarbons–Epoxides                                                   | 1 |
| 768 | Saturated hydrocarbons–Organic disulfides                                         | 1 |
| 769 | Alkyl halides–Other non-metal organides                                           | 1 |
| 770 | Alkyl halides–Organobromides                                                      | 1 |
| 771 | Saturated hydrocarbons–Tetralins                                                  | 1 |
| 772 | Phenanthrenes and derivatives–Naphthalenes                                        | 1 |
| 773 | Organic phosphoric acids and derivatives–Vinyl halides                            | 1 |
| 774 | Organic phosphoric acids and derivatives–Allyl-type 1,3-dipolar organic compounds | 1 |
| 775 | Phenols–Homogeneous other non-metal compounds                                     | 1 |
| 776 | Phenols–Tetralins                                                                 | 1 |
| 777 | Phenols–Organiodides                                                              | 1 |
| 778 | Phenols–Organobromides                                                            | 1 |
| 779 | Phenols–Other non-metal organides                                                 | 1 |
| 780 | Phenols–Anthracenes                                                               | 1 |
| 781 | Phenols–Carboximide acids and derivatives                                         | 1 |

|     |                                                                    |   |
|-----|--------------------------------------------------------------------|---|
| 782 | Phenanthrenes and derivatives–Phenol ethers                        | 1 |
| 783 | Organooxygen compounds–Carboximidic acids and derivatives          | 1 |
| 784 | Saturated hydrocarbons–Trialkylphosphites                          | 1 |
| 785 | Saturated hydrocarbons–Organic phosphoric acids and derivatives    | 1 |
| 786 | Saturated hydrocarbons–Organic carbonic acids and derivatives      | 1 |
| 787 | Organochlorides–Phenol ethers                                      | 1 |
| 788 | Naphthalenes–Carboximidic acids and derivatives                    | 1 |
| 789 | Naphthalenes–Oxazinanones                                          | 1 |
| 790 | Naphthalenes–Organoiodides                                         | 1 |
| 791 | Naphthalenes–Organobromides                                        | 1 |
| 792 | Naphthalenes–Dioxanes                                              | 1 |
| 793 | Organoiodides–Organochlorides                                      | 1 |
| 794 | Saturated hydrocarbons–Phenanthrenes and derivatives               | 1 |
| 795 | Lactones–NA                                                        | 1 |
| 796 | NA–Heteroaromatic compounds                                        | 1 |
| 797 | Stilbenes–Saturated hydrocarbons                                   | 1 |
| 798 | Organochlorides–Pyridines and derivatives                          | 1 |
| 799 | Organobromides–Unsaturated hydrocarbons                            | 1 |
| 800 | Organochlorides–Organofluorides                                    | 1 |
| 801 | Organofluorides–Prenol lipids                                      | 1 |
| 802 | Organofluorides–Fatty Acyls                                        | 1 |
| 803 | Organic oxoanionic compounds–Organooxygen compounds                | 1 |
| 804 | Organic oxoanionic compounds–Organoiodides                         | 1 |
| 805 | Dioxolanes–Homogeneous other non-metal compounds                   | 1 |
| 806 | NA–Tetrahydrofurans                                                | 1 |
| 807 | Organofluorides–Organochlorides                                    | 1 |
| 808 | NA–Vinyl halides                                                   | 1 |
| 809 | NA–Dioxanes                                                        | 1 |
| 810 | Polycyclic hydrocarbons–NA                                         | 1 |
| 811 | Polycyclic hydrocarbons–Benzene and substituted derivatives        | 1 |
| 812 | Other non-metal organides–Homogeneous other non-metal compounds    | 1 |
| 813 | Other non-metal organides–Allyl-type 1,3-dipolar organic compounds | 1 |
| 814 | Other non-metal organides–Organofluorides                          | 1 |
| 815 | Other non-metal organides–Dioxanes                                 | 1 |
| 816 | Lactones–Allyl-type 1,3-dipolar organic compounds                  | 1 |
| 817 | Stilbenes–Unsaturated hydrocarbons                                 | 1 |

|     |                                                           |   |
|-----|-----------------------------------------------------------|---|
| 818 | Organofluorides–Tetrahydrofurans                          | 1 |
| 819 | Saturated hydrocarbons–Anthracenes                        | 1 |
| 820 | Vinyl halides–NA                                          | 1 |
| 821 | Tetrahydrofurans–Homogeneous other non-metal compounds    | 1 |
| 822 | Tetrahydrofurans–Organo-post-transition metal compounds   | 1 |
| 823 | Tetrahydrofurans–Allyl-type 1,3-dipolar organic compounds | 1 |
| 824 | Tetrahydrofurans–Organiodides                             | 1 |
| 825 | Tetrahydrofurans–Organofluorides                          | 1 |
| 826 | Tetrahydrofurans–Organochlorides                          | 1 |
| 827 | Tetrahydrofurans–Organonitrogen compounds                 | 1 |
| 828 | Tetrahydrofurans–Fatty Acyls                              | 1 |
| 829 | Tetrahydrofurans–Dioxanes                                 | 1 |
| 830 | Vinyl halides–Sulfoxides                                  | 1 |
| 831 | Organobromides–Dioxanes                                   | 1 |
| 832 | Vinyl halides–Pyridines and derivatives                   | 1 |
| 833 | Vinyl halides–Carboxylic acids and derivatives            | 1 |
| 834 | Vinyl halides–Dioxanes                                    | 1 |
| 835 | Naphthalenes–Heteroaromatic compounds                     | 1 |
| 836 | Naphthalenes–Tetrahydrofurans                             | 1 |
| 837 | Organonitrogen compounds–Fatty Acyls                      | 1 |
| 838 | Allyl-type 1,3-dipolar organic compounds–Dioxanes         | 1 |
| 839 | Organobromides–Allyl-type 1,3-dipolar organic compounds   | 1 |
| 840 | Organobromides–Organooxygen compounds                     | 1 |
| 841 | Homogeneous other non-metal compounds–Oxathiolanes        | 1 |

## References

- [1] Yannick Djoumbou Feunang, Roman Eisner, Craig Knox, Leonid Chepelev, Janna Hastings, Gareth Owen, Eoin Fahy, Christoph Steinbeck, Shankar Subramanian, Evan Bolton, et al. Classyfire: automated chemical classification with a comprehensive, computable taxonomy. *Journal of cheminformatics*, 8(1):1–20, 2016.
- [2] Takuya Akiba, Shotaro Sano, Toshihiko Yanase, Takeru Ohta, and Masanori Koyama. Optuna: A next-generation hyperparameter optimization framework. In *Proceedings of the 25rd ACM SIGKDD International Conference on Knowledge Discovery and Data Mining*, 2019.
